# Supplementary material for: Finite-Time Analysis of Asynchronous Q-learning under Diminishing Step-Size from Control-Theoretic View
Source: arXiv:2207.12217 source file (2022-07-25)
Supplement: Supplementary file 1 [file convergence_rate.tex]

{\color{teal}
Here we hide factors other than number of time steps to see the if the probability tail bound leads to convergence rate. We replace the constants with the notation \(c, c_1\) and \(c_2\).

\begin{lemma}[\Cite{li2020sample}]\label{li:hi-exp}
Under adaptive learning rule~\eqref{li:step-size} and with slight modification of the Q-learning update, with probability \( 1- \delta \), the following bound is achieved:
\begin{align*}
    \mathbb{P}\left(||Q_k - Q^*||_{\infty} \leq c \sqrt{\frac{\log \left(\frac{k}{\delta}\right)\log k}{k} } \right) \leq \epsilon,
\end{align*}
where \(c\) is some constant.
The probability tail bound implies:
\begin{align*}
     \mathbb{E}\left[||Q_k-Q^*||_{\infty}\right] \leq   \frac{\sqrt{\pi}}{2} c \sqrt{ k\log k}.
\end{align*}
\end{lemma}
\begin{proof}
With probabiilty \( 1- \delta \),~\Cite{li2020sample} derives the following probability tail bound:
\begin{align*}
    \mathbb{P}\left(||Q_k - Q^*||_{\infty} \leq c \sqrt{\frac{\log \left(\frac{k}{\delta}\right)\log k}{k} } \right) \leq \epsilon.
\end{align*}
Using the popular translation method of probability tail bound to expectation~\Cite{chen2021lyapunov}, we have:
\begin{align*}
    \mathbb{E}\left[||Q_k-Q^*||_{\infty}\right] 
    &\leq \int^{\infty}_0 \mathbb{P} \left(||Q_k-Q^*||_{\infty} > x \right) dx \\
    &\leq  \int^{\infty}_0 k\exp\left(-\frac{x^2}{c^2} \frac{k}{\log k}\right) dx \\
    &=  \frac{\sqrt{\pi}}{2} c \sqrt{ k\log k}.
\end{align*}

The second inequality follows from expressing \(\delta\) in terms of \(x\):
\begin{align*}
    c \sqrt{\frac{\log \left( \frac{k}{\delta}\right) \log k}{k} } &= x\\
    \log \frac{k}{\delta} &= \frac{x^2}{c^2} \frac{k}{\log k} \\
    \frac{k}{\delta} &= \exp\left(\frac{x^2}{c^2} \frac{k}{\log k}\right) \\
    \delta &= k \exp\left(-\frac{x^2}{c^2} \frac{k}{\log k}\right).
\end{align*}
The last inequality follows form the fact that
\begin{align*}
    \int^{\infty}_0 e^{-x^2} = \frac{\sqrt{\pi}}{2}.
\end{align*}
This completes the proof.
\end{proof}

\begin{lemma}[\Cite{qu2020finite}]\label{qu:hp-ex}
The asynchronous Q-learning with step-size mentioned in~\Cref{sec:compare}, leads to following tail bound with probability \( 1 - \delta \):
\begin{align}
    \mathbb{P}\left(||Q_k - Q^*||_{\infty} \leq \frac{c_1}{k}+c_2\sqrt{ \frac{\log \frac{k^2}{\delta}}{k}}  \right) \leq \epsilon \nonumber
\end{align}
where \(c_1\) and \(c_2\) are some constant. It implies the following bound in expectation:
\vspace{1em}
  \setlength{\abovedisplayskip}{0pt}%
  \setlength{\belowdisplayskip}{0pt}%
  \setlength{\abovedisplayshortskip}{0pt}%
  \setlength{\belowdisplayshortskip}{0pt}
\begin{align*}
    \mathbb{E}[||Q_k-Q^*||_{\infty}] \leq \frac{c_1}{k}  + \frac{\sqrt{\pi}}{2c_2} k^{\frac{3}{2}}+\epsilon.
\end{align*}

\end{lemma}
\vspace{-5em}
\begin{proof}
We use the same techinque as in~\Cref{li:hi-exp}.
\vspace{1em}
  \setlength{\abovedisplayskip}{0pt}%
  \setlength{\belowdisplayskip}{0pt}%
  \setlength{\abovedisplayshortskip}{0pt}%
  \setlength{\belowdisplayshortskip}{0pt}
\begin{align*}
  \mathbb{E}\left[||Q_k-Q^*||_{\infty} - \frac{c_1}{k} - \epsilon\right]  &\leq \int^{\infty}_0 \mathbb{P}\left(||Q_k - Q^*||_{\infty} - \frac{c}{k} -\epsilon \geq x\right)\\
    &\leq  \int^{\infty}_0 k^2 \exp(-c_2^2kx^2) dx\\
    &= \frac{\sqrt{\pi}}{2c_2} k^{\frac{3}{2}}.
\end{align*}
\vspace{1em}
The last inequality follows from the following transformation of \( \delta \) to \(x\):
\vspace{1em}
  \setlength{\abovedisplayskip}{0pt}%
  \setlength{\belowdisplayskip}{0pt}%
  \setlength{\abovedisplayshortskip}{0pt}%
  \setlength{\belowdisplayshortskip}{0pt}
\begin{align*}
   \sqrt{ \frac{\log \frac{k^2}{\delta}}{k}}  &= c_2 x\\
    \log \frac{k^2}{\delta} &= c_2^2x^2 k\\
    \delta &= \frac{k^2}{\exp(c_2^2 x^2k)}.
\end{align*}
This completes the proof.
\end{proof}
}
